# Supplementary material for: Spin liquid fingerprints in the thermal transport of a Kitaev-Heisenberg ladder
Source: arXiv:1806.02344 ancillary file (2018-06-06)
Supplement: Supplementary file 1 [file Supp_Materials_Kitaev.pdf]

# Supplemental Material for
# Spin liquid fingerprints in the thermal transport of a Kitaev-Heisenberg ladder

Alexandros Metavitsiadis,[1] Christina Psaroudaki,[2] and Wolfram Brenig[1]

[1]*Institute for Theoretical Physics, Technical University Braunschweig, D-38106 Braunschweig, Germany*
[2]*Department of Physics, University of Basel, Klingelbergstrasse 82, 4056 Basel, Switzerland*

(Dated: June 5, 2018)

## A. RUNG SINGLET PERTURBATION

This section is devoted to the calculation of the low-lying excitations of the system in the limit of strong rung Heisenberg interaction $J'_H$. To begin with, we first consider the Hamiltonian of decoupled dimers

$$H_R = J'_H \sum_{i=1}^{N} \mathbf{S}_i^A \cdot \mathbf{S}_i^B \,, \tag{1}$$

where $\mathbf{S}_i^{A,B}$ denotes spin-1/2 operators located at the $i$-th site of the $A$ or $B$ chain of a ladder, correspondingly. In the absence of other interactions, the ground state of each dimer is a spin-singlet $|0,0\rangle_i = \frac{1}{\sqrt{2}}(|\uparrow\rangle_i^A|\downarrow\rangle_i^B - |\downarrow\rangle_i^A|\uparrow\rangle_i^B)$ with energy $E_0^{\text{rung}} = -3/4$. Thus, the ground state of the ladder is a direct product of spin-singlet states

$$|GS\rangle = |0,0\rangle_1|0,0\rangle_2 \cdots |0,0\rangle_N = \prod_{i=1}^{N} |0,0\rangle_i \,, \tag{2}$$

with energy $E^{\text{GS}} = NJ'_H E_0^{\text{rung}} = -3/4 J'_H N$. The excited states at each rung are spin triplet states $|1,1\rangle_i = |\uparrow\rangle_i^A|\uparrow\rangle_i^B$, $|1,-1\rangle_i = |\downarrow\rangle_i^A|\downarrow\rangle_i^B$ and $|1,0\rangle_i = \frac{1}{\sqrt{2}}(|\uparrow\rangle_i^A|\downarrow\rangle_i^B + |\downarrow\rangle_i^A|\uparrow\rangle_i^B)$ with energy $E_1^{\text{rung}} = 1/4$.

In the following, we consider the effect of coupling the dimers via a Heisenberg leg-Hamiltonian $H_H$ with coupling $J_H$ as well as a Kitaev leg-Hamiltonian $H_K$ with coupling $J_K$ in the limit $J'_H \gg J_H$ and $J'_H \gg J_K$. Hamiltonians $H_H$ and $H_K$ are defined below. We carry out a strong coupling expansion in which $H_R/J'_H$ is treated as the zeroth-order Hamiltonian, whereas the terms $H_{H,K}/J'_H$ are treated as small perturbations within a systematic expansion in terms of $J_{H,K}/J'_H$ . We use a derivation in close analogy with Ref.[1] where the strong coupling expansion was performed for the $S = 1$ chain with strong planar anisotropy.

### Heisenberg leg interactions

We first analyze the ground state and low-lying excitations in the presence of the perturbing Heisenberg Hamiltonian

$$H/J'_H = H_R/J'_H + H_H/J'_H = \sum_{i=1}^{N} \mathbf{S}_i^A \cdot \mathbf{S}_i^B + \frac{J_H}{J'_H} \sum_{i=1}^{N} \sum_{\alpha=A}^{B} \mathbf{S}_i^\alpha \cdot \mathbf{S}_{i+1}^\alpha \,. \tag{3}$$

Each bond of the perturbing Hamiltonian excites two adjacent singlets of the unperturbed ground state $|GS\rangle$ given in Eq. (2) to spin-1 triplet states, while the sum of the total $S_z$ quantum number is zero. The ground state including the first order correction is given by

$$\begin{aligned} |GS\rangle_H &= |GS\rangle + |\delta GS\rangle_H \\ &= |GS\rangle - \frac{J_H}{4J'_H} \sum_{i=1}^{N} (|1,0\rangle_i|1,0\rangle_{i+1} - |1,1\rangle_i|1,-1\rangle_{i+1} - |1,-1\rangle_i|1,1\rangle_{i+1}) \prod_{j\neq i,i+1} |0,0\rangle_j \,, \end{aligned} \tag{4}$$

while the ground state energy up to second order in $J_H/J'_H$ is $E_0^H = E_0 - {}_H\langle \delta GS|\delta GS\rangle_H = -\frac{3}{4}J'_H N - \frac{3}{8}\frac{J_H^2}{J'_H}N$. Higher order corrections are straightforward and have been evaluated in Ref. [2] where it has been found that the ground state energy up to third-order is $E_0^H = -\frac{3}{4}J'_H N - \frac{3}{8}\frac{J_H^2}{J'_H}N - \frac{3}{16}\frac{J_H^3}{(J'_H)^2}N$.

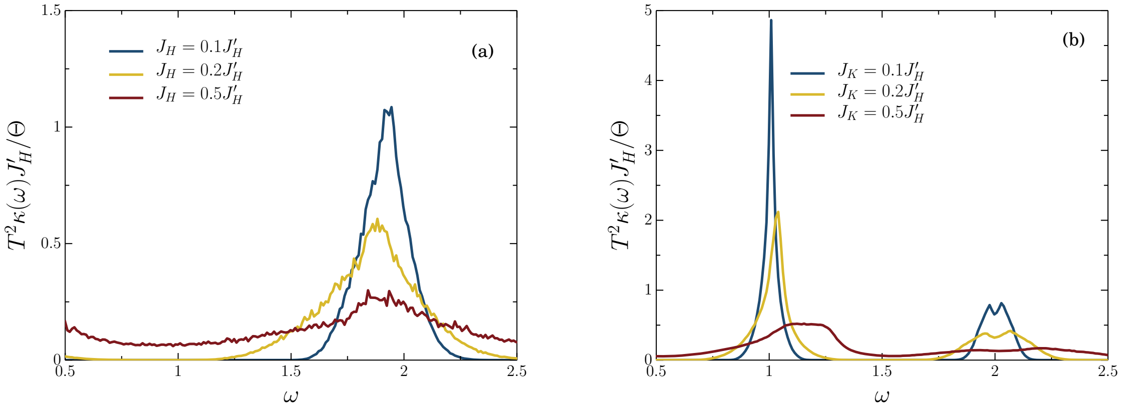


FIG. 1. High frequency part of the high temperature thermal conductivity for a Heisenberg (a) and Kitaev (b) ladder with $L = 8$ rungs for $J_H/J'_H = 0.1, 0.2, 0.5$ or $J_K/J'_H = 0.1, 0.2, 0.5$. We refer the reader to the main text of the present publication for definitions of the thermal conductivity $\kappa(\omega)$.

The first excited state of the unperturbed ladder is $3N$-fold degenerate and is obtained by promoting one rung to a triplet state $|s\rangle_n = |1, s\rangle_n \prod_{j\neq n} |0, 0\rangle_j$, with $s = 0, \pm 1$. States $|s\rangle_n$ are eigenstates of $H_R$ with energy equal to $E_0^{\rm tr} = J'_H(1 - \frac{3}{4}N)$ for any $n$. $H_H$ has the effect of moving the rung excitation to nearest-neighbor rungs, thus the degeneracy is removed by constructing states with definite crystal momentum

$$|k, s\rangle = \frac{1}{\sqrt{N}} \sum_{n=1}^{N} e^{ikn} |s\rangle_n \,. \tag{5}$$

We shall refer to states (5) as triplons to describe a non-localized triplet excitation. The first order correction of the triplon energy is found to be equal to $E^{\rm tr}(k) = \frac{1}{J'_H}\langle k, s|H_H|k, s\rangle = \frac{J_H}{J'_H}\cos(k)$. Thus, the excitation energy of the triplons up to first order is

$$\omega_H(k) = E_0^{\rm tr} + E^{\rm tr}(k) - E_0 = J'_H + J_H \cos(k)\,. \tag{6}$$

Higher order corrections are obtained through non-degenerate perturbation theory [2] and are found equal to

$$\omega_H(k) = J'_H + J_H \cos(k) + \frac{1}{4}\frac{J_H^2}{J'_H}(3 - \cos(2k)) - \frac{1}{8}\frac{J_H^3}{(J'_H)^2}(2\cos(k) + 2\cos(2k) - \cos(3k) - 3)\;. \tag{7}$$

We note that the single triplon dispersion relation has a minimum at $k = \pm\pi$.

We now turn our attention to two-body states, namely states with total magnetization $M = \pm 2$ consisted of two-triplons with $S_z = \pm 1$ correspondingly, states with $M = \pm 1$ consisted of one triplon with $S_z = 0$ and one with $S_z = \pm 1$ and states with $M = 0$, consisted of either two triplons with $S_z = 0$ or one triplon with $S_z = 1$ and one with $S_z = -1$. First we note that since the triplon states are degenerate, the excitation energy of any two-body state with one triplon with crystal momentum $k_1$ and one with $k_2$ fall into a two-body continuum with energies $\Omega_H^{M=\pm 2}(k_1, k_2) = \omega_H(k_1) + \omega_H(k_2)$. Folding the wavevector $k = k_1 + k_2$ to the first Brillouin zone $[-\pi, \pi]$, the continuum extends between the two boundaries

$$\Omega_H(k) = 2J'_H \pm 2J_H \cos(k/2)\,, \tag{8}$$

expressed up to first order in $J_H/J'_H$. Although the two-body continuum energies are the same for any two-body state, the two-triplon bound state energy is expected to depend on the $M$ sector. Following the calculations of Ref. [1] for the $S = 1$ chain based on an elementary Bethe ansatz, we find that the bound state energy of the $M = \pm 2$ sector is equal to $\Omega_H^{M=\pm 2}(k) = 2J'_H + J_H\left(\frac{1}{2} + 2\cos(k/2)^2\right)$ which exists when $2\pi/3 \leq |k| \leq \pi$, lies above the continuum and merges with it at the cut-off momentum $2\pi/3$. Similarly for $M = \pm 1$ we find $\Omega_H^{M=\pm 1}(k) = 2J'_H - J_H\left(\frac{1}{2} + 2\cos(k/2)^2\right)$, which lies below the continuum between wavevectors $2\pi/3 \leq |k| \leq \pi$ and finally for $M = 0$ the bound state energy is $\Omega_H^{M=0}(k) = 2J'_H - J_H\left(1 + \cos(k/2)^2\right)$ which is stable for the whole zone $0 \leq |k| \leq \pi$. We note that in Ref. [3], analytical expressions for the bound states of sector $M = 0$ and $M = 1$ are derived based on a mapping of the model

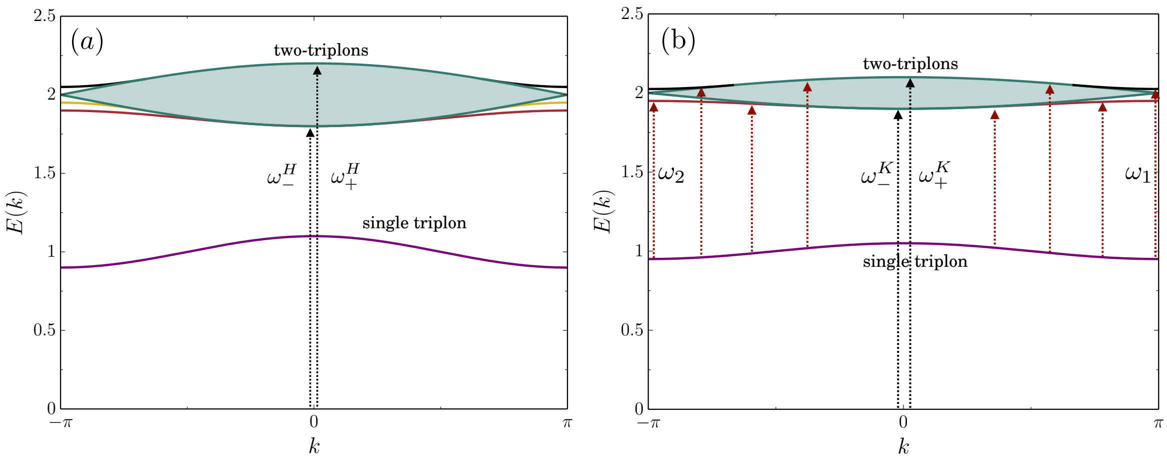


FIG. 2. (a) One- and two-particle excitation spectrum for the Heisenberg leg model with $J_H/J'_H = 0.1$. Solid lines correspond to the single triplon (purple), the $M = 0$ bound state (red), the $M = \pm 1$ bound state (yellow) and the $M = \pm 2$ bound state (black). The two-triplon continuum is depicted by the green colored surface. Frequencies $\omega_\pm^H$ (dashed arrows) correspond to the boundary lines of the high-frequency band of $\kappa(\omega)$. (b) One- and two-particle excitation spectrum for the Kitaev leg model with $J_K/J'_H = 0.1$. Solid lines correspond to the single triplon (purple), the $M = 0$ bound state (red) and the $M = \pm 2$ bound state (black). The two-triplon continuum is depicted by the green colored surface. Frequencies $\omega_\pm^K$ (black dashed arrows) correspond to the boundary lines of the high-frequency band of $\kappa(\omega)$, while red dashed lines indicate some of the allowed transitions for the low-frequency band of $\kappa(\omega)$. Among them most of the intensity arises from the $k = \pm\pi$ boundary at frequencies $\omega_{1,2}$.

onto a Bose gas of hard-core triplets. The one- and two-particle excitation spectrum of the Heisenberg leg Hamiltonian (3) are presented in Fig. 2(a) for $J_H/J'_H = 0.1$.

We note that the matrix elements $\langle n|j^\epsilon|m\rangle$ are non-vanishing for states $|n\rangle$, $|m\rangle$ that obey the selection rules $\Delta S_z = 0$ and $\Delta k = 0$. In addition, assuming that the dominant contribution in the thermal conductivity $\kappa(\omega)$ originate from the ground state $|GS\rangle_H$ to other excited states, we note that the operation $j^\epsilon|GS\rangle_H$ generates a state which belongs to the manifold of states with two excited triplons. Thus, the only possible transitions are between the ground state and the two-triplon continuum (of two $S_z = 0$ triplons or a pair of $S_z = 1$ and $S_z = -1$ triplons) at $k = 0$ which results contributions from a band of frequencies with boundary lines $\omega_\pm^H = 2J'_H \pm 2J_H$. A simple inspection of Fig. 1(a) reveals that in the high temperature limit most of the intensity is concentrated near the $\omega_-^H$ limit which is likely due to the fact that it involves transitions to the two-triplon continuum at its lowest gap and is thus more heavily populated. This is further confirmed by the shifting of the band to lower frequencies as the Heisenberg coupling $J_H$ is increased. Bound states branch off the continuum near the zone boundary and are not expected to give a distinct signal in the thermal conductivity. Finally, the operation $j^\epsilon|k,s\rangle$ yields states with three excited triplons, thus we do not observe any contribution coming from transitions between single and two triplons.

### Kitaev leg interactions

The remainder of this section is devoted in the analysis of the low-lying excitation spectrum in the presence of the perturbing Kitaev Hamiltonian

$$H/J'_H = H_R/J'_H + H_K/J'_H = \sum_{i=1}^{N} \mathbf{S}_i^A \cdot \mathbf{S}_i^B + \frac{J_K}{J'_H}\sum_{i=1}^{N/2}(S_{2i,A}^x S_{2i+1,A}^x + S_{2i,A}^y S_{2i-1,A}^y + S_{2i,B}^x S_{2i-1,B}^x + S_{2i,B}^y S_{2i+1,B}^y)\,. \tag{9}$$

Based on similar considerations like before we find that the first order correction the ground state is given by

$$|GS\rangle_K = |GS\rangle + \frac{J_K}{4J'_H}\sum_{l=0}^{N/2-1}\left(|1,1\rangle_{2l}|1,-1\rangle_{2l+1} + |1,-1\rangle_{2l}|1,1\rangle_{2l+1}\right)\prod_{j\neq 2l,2l+1}|0,0\rangle_j\,, \tag{10}$$

while the ground state energy up to second order in $J_K/J'_H$ is $E_0^K = -\frac{3}{4}J'_H N - \frac{3}{4}\frac{J_K^2}{J'_H}(\frac{N}{2} - 2)$. Moreover, we note that the Kitaev Hamiltonian lifts the degeneracy of the triplon modes with $S_z = \pm 1$ and the one with $S_z = 0$. More

specifically, the triplon excitation energy is

$$\omega^K_{\pm 1}(k) = J'_H + \frac{J_K}{2}\cos(k)\,, \qquad \omega^K_0 = J'_H\,, \tag{11}$$

up to first order in $J_K/J'_H$. In (11) we have omitted states that contain more than one excited rung, as is appropriate to leading order. We now turn our attention to two-triplon states, focusing first on two unbounded excitations. The boundaries of the two-body continuum consisted of any combination of two states with $S_z = \pm 1$ and wavevectors $k_1$ and $k_2$ are

$$\Omega_K(k) = 2J'_H \pm J_K\cos(k/2)\,, \tag{12}$$

with $k = k_1 + k_2$. A two-body state consisted of two $S_z = 0$ triplons is $N(N-1)/2$ degenerate with energy $\Omega^K_0 = 2J'_H$, while a two-body state consisted of one $S_z = 0$ triplon and one with $S_z = \pm 1$ triplon with crystal momentum $k$ has an excitation energy equal to $\Omega^K_1 = 2J'_H + J_K/2\cos(k)$. In addition, the bound state energy in the $M = \pm 2$ sector is $\Omega^{M=\pm 2}_K(k) = 2J'_H + J_K/2\left(\frac{1}{2} + 2\cos(k/2)^2\right)$ which exists when $2\pi/3 \leq |k| \leq \pi$ while the bound state energy of a triplon with $S_z = 1$ and one with $S_z = -1$ belonging in the $M = 0$ sector is $\Omega^{M=0}_K(k) = 2J'_H - J_K/2\left(1 + \cos(k/2)^2\right)$. The one- and two-particle excitation spectrum of the Kitaev leg Hamiltonian (9) are presented in Fig. 2(b) for $J_K/J'_H = 0.1$. We note that the calculation of bound states involving triplons with $S_z = 0$ is omitted because they lie for energies in-between the bound states energies of the $M = 0$ and $M = \pm 2$ sector and are not expected to give rise to prominent signals in the $\kappa(\omega)$. Their calculation relies on an involved degenerate perturbation theory.

The selection rules between states $|n\rangle$ and $|m\rangle$ to obtain non-vanishing matrix elements $\langle n|j^\epsilon|m\rangle$ depend on the symmetries of the Hamiltonian under study. We note that for the Kitaev Hamiltonian of Eq. (9) with less symmetries than the Heisenberg one, only the $\Delta k = 0$ rule needs to be fulfilled. As anticipated, the high-frequency part of $\kappa(\omega)$ contains contributions from the ground state to the two-particle sector from a band of frequencies with boundary lines $\omega^K_\pm = 2J'_H \pm J_K$. The most unexpected feature of Fig. 1 is an additional dominant signal for frequencies $\sim J'_H$ which is absent for the Heisenberg perturbation scheme and originates from transitions between excited states. More precisely, the operation $j^\epsilon|k, s\rangle$ generates states in the two-triplon manifold with energies given by the two-triplon continuum as well as the two-triplon bound states. To analyze the resulting signal we need to take into account that transitions are allowed for every $k$ in the first Brillouin zone $[-\pi, \pi]$ that will eventually produce a zoo of allowed frequencies given by the difference of the energies of the two-triplon and the single triplon states. To simplify the picture, we note that by increasing the Kitaev coupling $J_K$ the band shifts to higher frequencies, indicating the fact that most of the intensity arises from transitions at $k = \pm\pi$ where triplons have their lowest gap and are thus more populated. At $k = \pm\pi$ the frequency band lies between the lines $\omega_1 = \Omega^{M=\pm 2}_K(\pi) - \omega^K_{\pm 1}(\pi) = J'_H + 3J_K/4$ and $\omega_2 = \Omega^{M=0}_K(\pi) - \omega^K_{\pm 1}(\pi) = J'_H$.

In Fig. 3 we present the frequency dependence of the correlation function $\tilde{C}(\omega)J'_H/\Theta$, where

$$\tilde{C}(\omega) = \mathrm{Re}\frac{1}{L}\int_{-\infty}^{\infty}\frac{d\omega}{2\pi}e^{-i\omega t}\langle j^\epsilon(t)j^\epsilon\rangle\,, \quad \text{and} \quad \Theta = \frac{\pi}{L}\langle j^\epsilon j^\epsilon\rangle\,. \tag{13}$$

The correlation function $\tilde{C}(\omega)$ and the thermal conductivity defined in the main text are related as $\kappa(\omega) = \tilde{C}(\omega)\beta(1 - e^{-\beta\omega})/\omega$. While the latter vanishes for $\beta = 0$, the former displays the temperature dependence of the $J'_H$-mode in the whole temperature range, showing a clear decay of its weight with decreasing temperature and, as expected, the signal around $J'_H$ almost vanishes in the low temperature limit of $\beta = 5$.

[1] N. Papanicolaou and P. Spathis, J. Phys.: Condens. Matter **2** 6575 (1990).
[2] M. Reigrotzki, H Tsunetsugu and T. M. Rice, J. Phys.: Condens. Matter **6**, 9235 (1994).
[3] V. N. Kotov, O. P. Sushkov, and R. Eder, Phys. Rev. B **59** 6266 (1999).

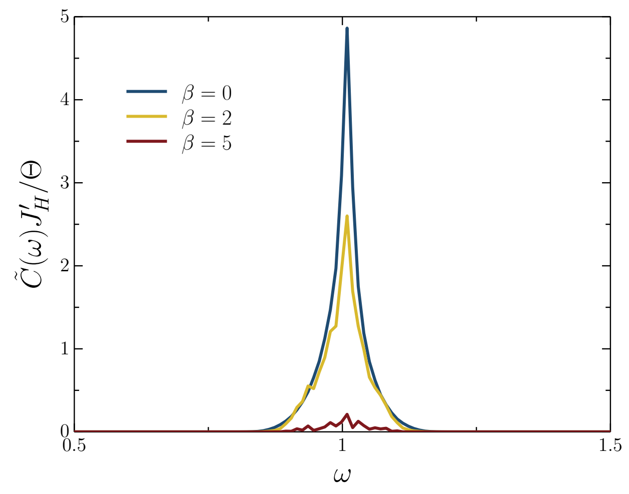


FIG. 3. Frequency dependence of the correlation function $\tilde{C}(\omega)J_H^{'}/\Theta$ around $\omega = 1$ of a Kitaev ladder with $L = 8$ rungs for $J_K/J'_H = 0.1$ and various values of the inverse temperatures $\beta$. In the low temperature limit of $\beta = 5$ we note that the dominant signal $\sim J'_H$ vanishes as expected, indicating that it originates from transitions between excited states.
